# Supplementary material for: Large Language Model Adversarial Landscape Through the Lens of Attack Objectives
Source: arXiv:2502.02960 source file (2025-02-05)
Supplement: Supplementary file 1 [file appendix.tex]

\appendix

\section{Data Availability}

We will comply with the data availability policy by openly sharing all relevant data associated with this manuscript on an open-source platform, such as GitHub, to ensure it contributes to the broader scientific community and maximizes its value.
